# Supplementary material for: ASIA: Adaptive 3D Segmentation using Few Image Annotations
Source: arXiv:2509.24288 source file (2025-09-29)
Supplement: Supplementary file 1 [file X_supplementary.tex]

% \newpage
% \clearpage
% \onecolumn
% \input{figures/comparison_2}
