# Supplementary material for: ASIA: Adaptive 3D Segmentation using Few Image Annotations
Source: arXiv:2509.24288 source file (2025-09-29)
Supplement: Supplementary file 2 [file failure_cases.tex]

\section{Failure Cases}
\label{sup_sec:failure_cases}

\begin{figure}[h]
    \includegraphics[width=0.9\linewidth]{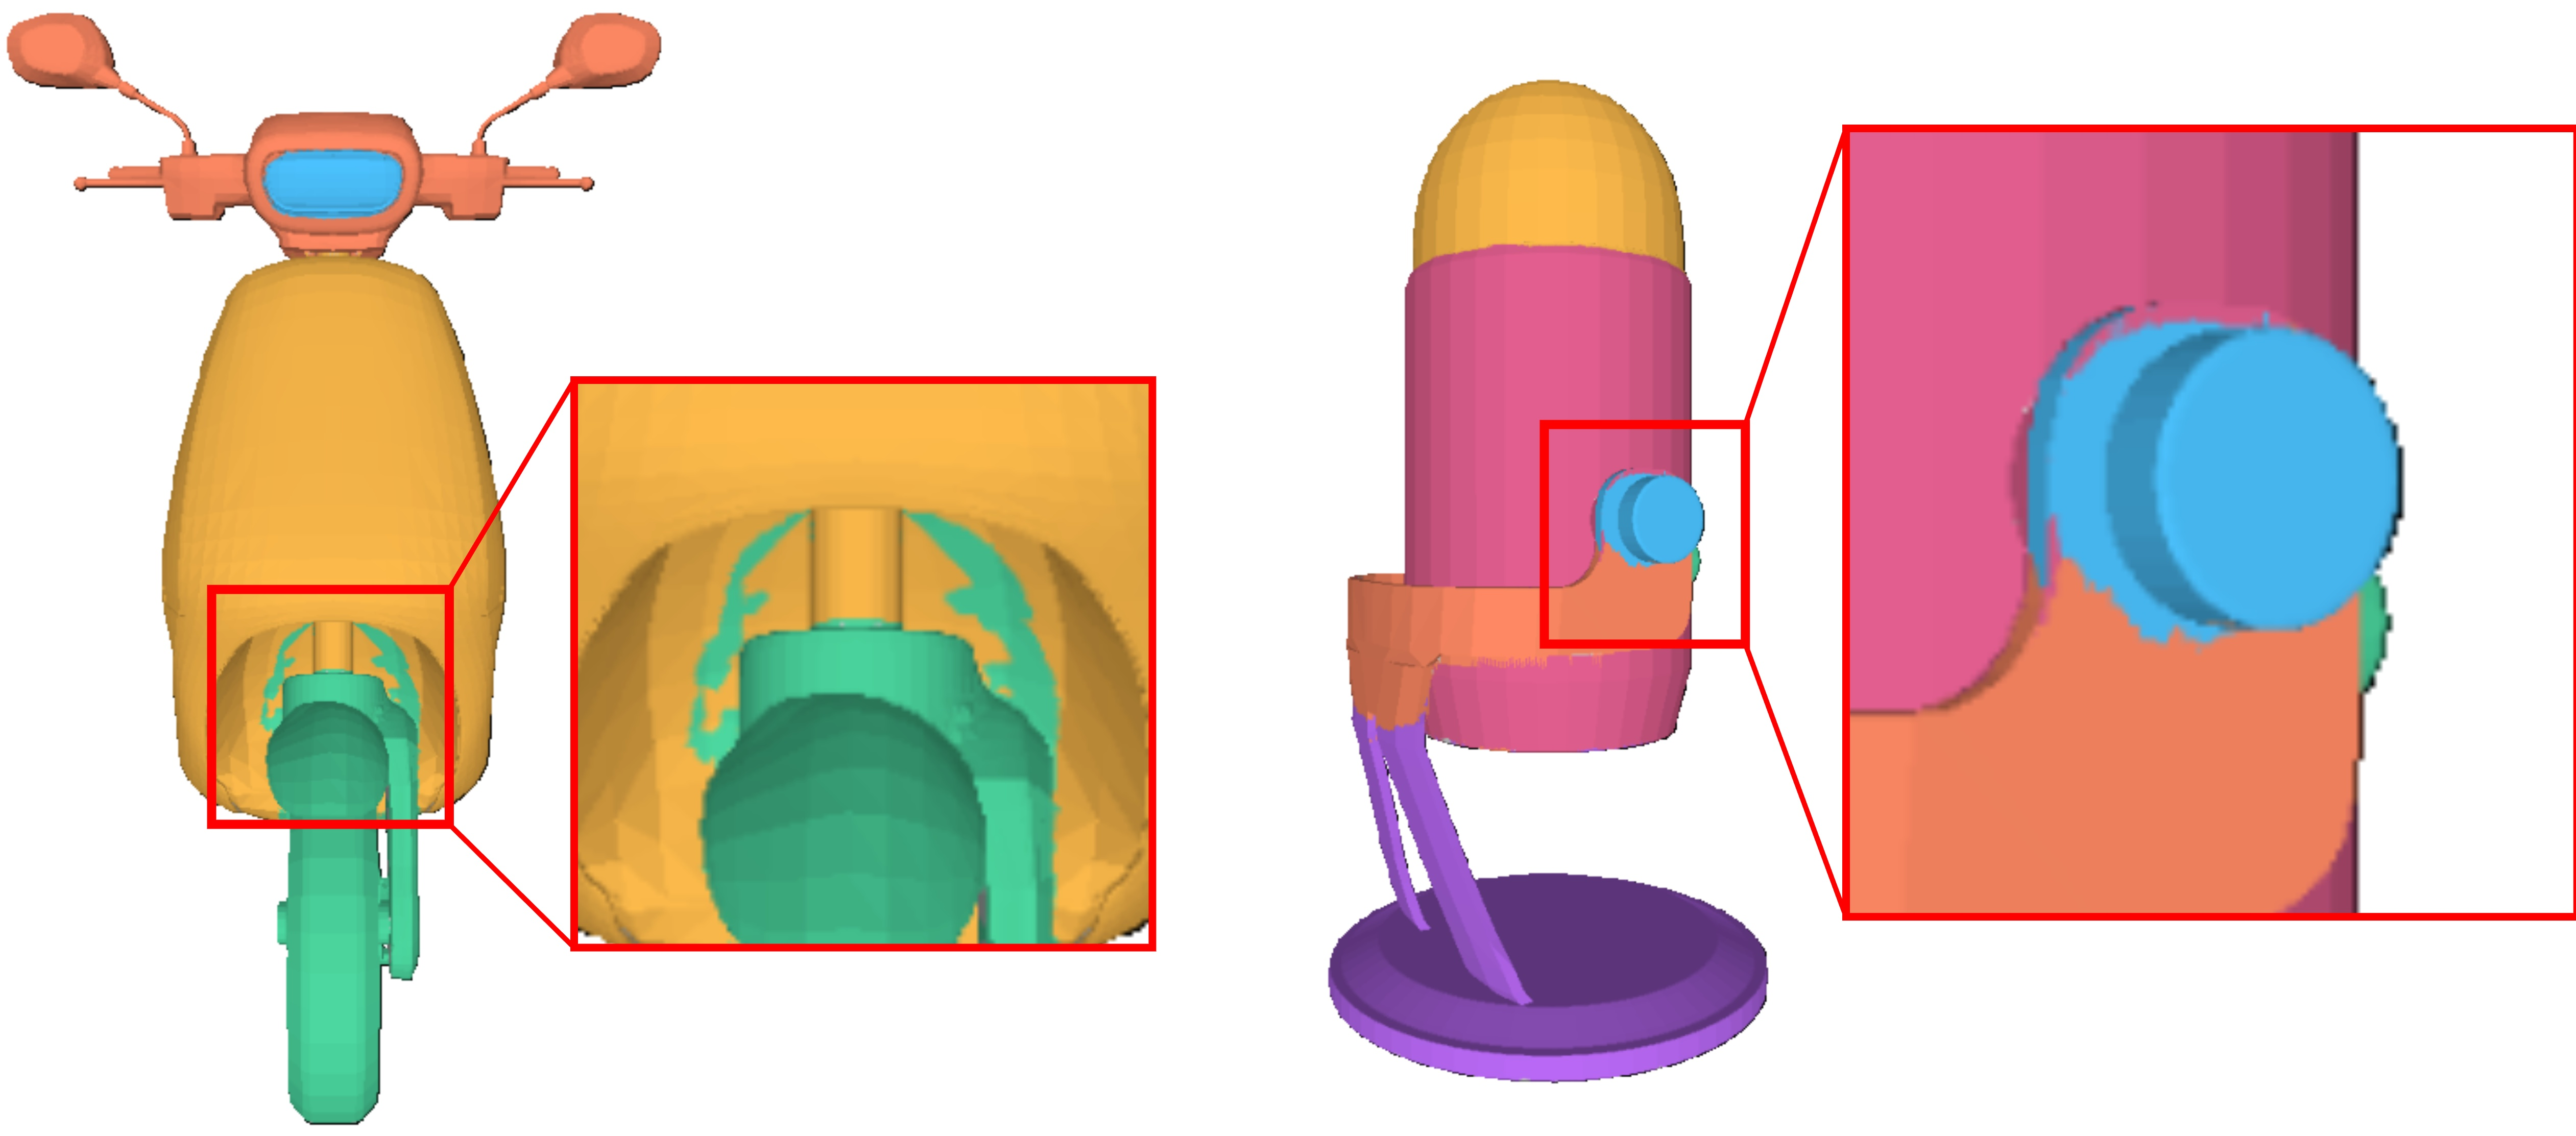}
  \caption{\textbf{Failure Cases.} Segmentation spillover can occasionally occur for small parts and low-confidence regions.}
  \label{fig:fail_case}
\end{figure}

Despite its strengths, our method has certain limitations—particularly in scenarios involving small parts or low-confidence regions, where the multi-view 2D predictions may fail to accurately localize the region of interest.
This issue becomes more pronounced when such regions overlap with other parts across different views during inference.
As a result, as illustrated in Fig.~\ref{fig:fail_case}, these overlaps can lead to segmentation spillover, where the predicted mask for one part incorrectly extends into adjacent or overlapping parts of the object, causing occasional inaccuracies in the final output.
