# Supplementary material for: ASIA: Adaptive 3D Segmentation using Few Image Annotations
Source: arXiv:2509.24288 source file (2025-09-29)
Supplement: Supplementary file 3 [file noise_opt_intuition.tex]

% NOTE: DO NOT INCLUDE THIS

\section{Intuition behind noise optimization}
\label{sup_sec:noise_opt_intuition}

\begin{itemize}
    \item When we ask SD to generate an image of a "red car", it generates an image following the prompt, as we vary the seed (i.e. vary the initial noise) it generates new images that still respect the prompt. However, the model might still not generate the exact car we want. 
    
    The same is with \textit{MV consistent segmentation} in our case, a random initial noise may lead to inconsistent results across views which may not be easily fixed by merely changing the seed. 
    
    \item Changing the seed will generate new results that still respect the optimized text prompt but may still not be perfect for us (i.e. not MV consistent).
    \saura{But reviewer can say , if i pass it in a batch i can also use the self-attention inflation to fix it, why noise will only fix the MV consistency ? }
    
    \item Noise optimization allows us to find the right initial noise (through optimization) for which segmentations across all views become consistent.
    
    \item Why it works? When we optimize noise, the globally aggregated segmentation map (obtained through voting) improves the individual predictions through optimization, which in turn improves the global prediction, and so on.

    \item Why it becomes more imporatnt for non-semantic segmentation? Semantic segments are obtained from emergent features of the Diffusion Model~\cite{namekata2024emerdiff}. However, non-semantic segments are harder to obtain from emergent properties, as a result the MV consistency of these segments is lower than that of semantic segments.

    Noise Optimization acts as an additional regularization, to improve the MV consistency for non-semantic segments. 

    \item There dosen't exists a unique noise that will give the best MV consistency and that we want to achieve through Noise Optimization.
    There can be many noises which can lead to the same result. This is mainly because of the way the diffusion model is trained. \saura{contradictory with 1st few points}
    \sr{[VERIFY!]}
\end{itemize}

% \begin{figure}[t]
%       \includegraphics[width=\linewidth, height=3.5cm]{example-image-a}
%   \caption{Intuition Figure.}
%   \Description{Teaser Figure.}
%   \label{fig:intuition}
% \end{figure}

\begin{figure}[t]
  \includegraphics[width=\linewidth]{images/noise.jpg}
  \caption{The effect and importance of noise optimization. Changing seed does not necessarily help with multiview consistency. Whereas Noise-Optimization makes the predictions consistent across views.}
  \Description{intuition}
  \label{fig:intuition}
\end{figure}
